# Supplementary material for: Faddeev Random Phase Approximation applied to molecules
Source: arXiv:1210.6186 source file (2012-10-23)
Supplement: Supplementary file 1 [file appendix.tex]

\chapter{Appendix}
\label{app:tango}

\section{Introduction}
