# Supplementary material for: Faddeev Random Phase Approximation applied to molecules
Source: arXiv:1210.6186 source file (2012-10-23)
Supplement: Supplementary file 2 [file Bijl.pdf]

Prof.dr.ir.drs. Hester Bijl  
Full professor Aerodynamics  
Faculty of Aerospace Engineering  
Delft University of Technology  
Kluyverweg 1  
2629 HS Delft  
The Netherlands

## **Evaluation of the PhD thesis of Joris Degroote entitled “Development of algorithms for the partitioned simulation of strongly coupled fluid-structure interactions”**

### *Summary*

The PhD-thesis concerns numerical solution of strongly coupled fluid-structure interactions. Partitioned solution of these problems is commonly chosen as existing solvers can be reused. However, obtaining a numerically stable solution is not trivial, especially for strongly coupled cases and when incompressible flows are involved. Also efficiency is of major importance, as these are computationally expensive unsteady problems, which might require a large number of sub-iterations in each time step.

In the thesis coupling algorithms are proposed, analyzed and applied to several fluid-structure interaction problems. After an extensive literature review in Chapter 2, in Chapter 3 stability of the Gauss-Seidel coupling method with various combinations of coupling terms is analyzed for unsteady, incompressible flow in a straight, flexible tube. In Chapter 4 two black box solvers the new quasi-Newton coupling method is introduced and used to couple two black box solvers. For two test problems performance is compared with several other partitioned methods and a monolithic method. In Chapter 5 a black box solver is coupled with an accessible solver. In the first part, bubble and droplet dynamics are simulated, while in the second part the interface artificial compressibility method is introduced. Chapter 6 concerns a study when different solvers, or meshes are used, while in Chapter 7 challenging fluid-structure interactions with free surface flows are discussed.

### *Assessment*

I recommend the thesis for public defense without any mandatory changes. The work is highly innovative and of very high quality. I am impressed by both the depth as well as the breadth. The stability analysis is new and provides new insights. In addition, new coupling techniques are proposed and their superiority is shown in extensive comparisons with existing methods. Finally, challenging fluid-structure interaction problems involving droplets and free surface are

computed as well. The thesis is well written and the literature survey is extensive. The publication list of the author is impressive.

### *Questions and suggestions*

I do not have any suggestions for changes to the thesis. I have a few topics which I would like to discuss during the first meeting. Some of them are:

#### 1. Stability analysis

##### a) Addition of coupling terms

On page 44 of Chapter 3 a stability analysis is performed of Gauss-Seidel partitioning, where information of the elastic wall is added to the flow equations in several places. Would it be possible to do it the other way around, add information on fluid pressures to the structure equation? What would the stability of that type of iteration be compared to the scheme analyzed in the thesis?

##### b) Dependence on boundary conditions

How are the boundary conditions taken into account in the stability analysis? Would a change of boundary conditions affect the result?

##### c) Dependence on discretization in space and time

What does the amplification factor for the monolithic system (not the  $\mu$  in Eq. (3.27), but the "standard" one for the discretization) look like? Is there significant damping for the high frequency modes caused by:

- the implicit Euler time integration
- the first order upwind spatial discretization
- the pressure stabilization

Does the fact that the partitioning is only unstable for low frequency modes depend on this damping of high frequency modes in the discretization? I.e. what would happen when a pure central discretization is used in combination with the trapezoidal rule and no stabilization term? In that case less damping is present for the high frequency modes present, will then also only the low frequency errors be unstable?

#### 2. Multi-solver and multi-level implementation

Do you have comparisons of MS implementations of IQN-ILS and IBQN-LS with regular implementations? I am interested in more information on the multi-level algorithm. Why did you choose to go from coarse to fine and not use a V-cycle? On page 179 a bias is mentioned in the results when certain terms are added to V and W. Where does this bias come from?

Sincerely,

Prof. Hester Bijl.
