# Supplementary material for: Faddeev Random Phase Approximation applied to molecules
Source: arXiv:1210.6186 source file (2012-10-23)
Supplement: Supplementary file 3 [file Geuzaine.pdf]

Gosselies, March 17, 2010

## **PhD evaluation of Joris Degroote**

### **“Development of Algorithms for the Partitioned Simulation of Strongly Coupled Fluid-Structure Interaction Problems”**

#### **Assessment**

The work is impressive. The thesis offers several original contributions to the field of the partitioned simulation of fluid-structure interaction problems involving incompressible flows and (very) flexible structures. The work is constructed with methodology: in depth stability analysis on some simplified model problems to understand the convergence problems associated with partitioned approaches, development of new algorithms based on the findings of the stability analysis, many benchmarks of the developed methods with respect to state-of-the-art ones (monolithic and partitioned), application to academic and engineering applications with in-house as well as commercial solvers. The thesis is well written and contains a very detailed and helpful literature overview. The list of publications associated with the thesis is impressive and shows the high quality of the work. Overall, the thesis demonstrates the solid background in (computational) fluid and structural dynamics of the author as well as his capacity to translate the developed algorithms into software. I therefore highly recommend the thesis for public defense.

#### **Questions/suggestions**

1. p 106: It would be interesting to see the performance of IQN-ILS with no use of previous time-steps.
2. p 112: How about the memory footprint in Table 4.4?
3. p 112: Could the author elaborate on the use of a limiter?
4. p 115: Could the author add some information for the “strong coupling” case?
5. p 145: It would be interesting to compare the results with a VOF approach.
6. p. 166: The license cost (serial vs. parallel) of commercial solvers could be added to the discussion related to the multisolver version of the algorithms.
7. p. 184: Does the multilevel version of the solvers prove to be more robust?
8. While the list of publications associated with the thesis is impressive, a section in the (introduction or conclusion of the) thesis could gather a summary with the main achievements of them.
9. A great emphasis has been put in developing coupling between black-box solvers. This is well motivated from a conceptual point of view. Is it the experience of the

- author that most solvers do not offer access through user-defined function so that the IAC algorithm (detailed and applied in Chap. 5) cannot be implemented?
10. The thesis focuses mainly on convergence issues. What would be the impact of replacing the first-order time-accurate approach by a second-order one in the flow solver?
  11. How could the approach be applied to fluid-thermal problems?
  12. As the main motivation for partitioned approaches is solver re-usability and the limitation of monolithic solvers to moderate size problems, it would have been nice to demonstrate on a large-scale problem (involving several millions of degrees of freedom) the advantage of partitioned approaches.

Sincerely,

Dr. Philippe Geuzaine
