# Supplementary material for: Faddeev Random Phase Approximation applied to molecules
Source: arXiv:1210.6186 source file (2012-10-23)
Supplement: Supplementary file 4 [file Segers.pdf]

**Your reference**

**Our reference**

**date**

05-03-2010

**Contact person**

**e-mail**

patrick.segers@UGent.be

**tel. and fax**

**T** +32 9 332 3466

**F** +32 9 332 4159

PhD thesis Joris DEGROOTE

*"Development of Algorithms for the Partitioned Simulation  
of Strongly Coupled Fluid-Structure Interaction Problems"*

report by Patrick Segers

In this work, Joris Degroote introduces and applies a number of refinements to existing and new algorithms to couple black-box numerical solvers for the fluid and structure problem in fluid-structure interaction simulations. This partitioned approach stands in contrast with the so-called monolithic approach where the flow and structural equations are solved simultaneously. The partitioned approach offers the advantage that dedicated flow and structural solvers can be used (which are commonly more advanced, allowing to solve complex fluid or structural mechanical problems), but has the disadvantage that (iterative) coupling between the two solvers is required to find a solution which satisfies both the structural and flow equations at the fluid-structure interface boundary, a non-trivial problem. In this dissertation, multiple strategies are discussed and have been developed to resolve this iteration problem.

Following the introduction chapter, chapter 2 provides a literature overview, mainly focusing on partitioned approaches, and clearly delineating between explicit (weakly coupled) and implicit (strongly coupled) techniques. It is clear from this chapter that the candidate has a profound and fundamental insight into this research domain which he totally masters, with an in my perception very complete overview of different strategies, and with an excellent referral to the literature. In chapter 3, a stability analysis of Gauss-Seidel iterations is provided for the case of pulsatile flow in a flexible tube (as model of blood flow in an artery), using an innovative Fourier-based approach. It is demonstrated that the instability of the Gauss-Seidel iterations increases with increasing distensibility of the tube, and, less intuitively clear, when the time step decreases. Adding mass to the structure and accounting for inertial effects of the structure has as stabilizing effect on the simulations.

Chapter 4 focuses on strategies coupling two black box solvers (such as Fluent and Abaqus). A new method is introduced, called IQN-ILS (calculating the displacement of the interface using quasi-Newton iterations with an approximation of the inverse of the Jacobian from a least squares model). The performance is compared to other existing and modified partitioned methods, including the IBQN-LS method (Interface block quasi-Newton with approximate Jacobian from least squares models), Aitken

relaxation and Interface-GMRES (Interface generalized minimal residual) using 2 numerical experiments (flexible beam and flexible tube). For the chosen examples, IQN-ILS performs similarly as IBQN-LS, and better than the two other methods. In this chapter, IQN-ILS is also compared with a monolithic approach for different cases. Which method performs best depends on the case studied. The monolithic approach converges faster in most –but not all – cases.

Chapter 5 deals with the case where either the structural solver, either the flow solver is accessible. The problem of bubble and droplet dynamics is solved for the case of an accessible structural solver, while the problem of wave propagation in a (bifurcating) tube is solved for the case of an accessible fluid solver. The latter consists of implementation of the interface artificial compressibility (IAC) method and has been applied to the simulation of wave propagation in a straight artery as well as a carotid bifurcation. In both cases, IAC was the fastest technique when compared with the IBQN-LS method. When simulating a flexible beam, however, the IBQN-LS proved the fastest technique.

In chapter 6, some of the previously described techniques are implemented using a multi-solver or multi-level approach to make optimal use of parallelization and available computer power in cluster configurations. In chapter 7, a fluid-structure interaction problem with free surface flow is solved for the case of a rolling tank, partially filled with a liquid, which interacts with a flexible beam. The agreement with experimental data is, overall, good. A final application is the simulation of a composite cylinder, falling on the free water surface, demonstrating the importance of design parameters (stiff versus flexible cylinder) on stresses arising during the impact. For both applications, IQN-ILS is compared with Aitken relaxation techniques, the former being the fastest technique. In Chapter 8, some general conclusions and recommendations for future work are given.

Overall, the PhD-thesis of Joris Degroote is of an exceptionally high level. Most of the work has been or will be published in >10 papers in peer-reviewed journals. I recommend to give Joris Degroote unconditional permission to the public defence.

Some minor editorial comments/suggestions:

- I would suggest to also explain the acronyms in the summary
- Page xiii: “slagader” instead of “ader”
- Typo p18: .. and that the pressure...
- Typo p81: start par 2: Newtons
- Typo p102: ..However, its calculation (instead of it's)
- Section 5.2.1.: add a figure to introduce the coordinate system ?
- Figure 5.6:  $P_E$  should be  $P_1$  ?
- P167: for  $i = \dots$  (instead of  $0 = \dots$ )

Sincerely,

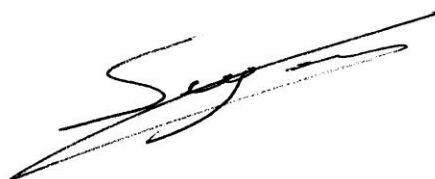

prof. dr. ir. Patrick Segers  
Gent, March 5th, 2010
