# Supplementary material for: Faddeev Random Phase Approximation applied to molecules
Source: arXiv:1210.6186 source file (2012-10-23)
Supplement: Supplementary file 5 [file VanPaepegem.pdf]

**Prof. dr. ir. L. Taerwe**  
Dean of the Faculty of Engineering  
Sint-Pietersnieuwstraat 41  
9000 Gent

**date**  
14 March 2010

**contact**  
Wim VAN PAEPEGEM

**e-mail**  
Wim.VanPaepegem@UGent.be

**phone and fax**  
T +32 9 264 42 07  
F +32 9 264 35 87

**Evaluation report on the PhD dissertation of  
ir. Joris DEGROOTE entitled  
“Development of algorithms for the partitioned simulation of  
strongly coupled fluid-structure interaction problems”**

This PhD thesis presents the development of new algorithms for the partitioned simulation of strongly coupled fluid-structure interaction problems. This topic is receiving a lot of international attention nowadays, as realistic simulation of complicated fluid-structure interaction problems is getting more and more feasible, due to improved CFD and FEA codes, and very cheap computational power.

***Overall appreciation***

I highly appreciated this work in terms of scientific originality, the profound approach of all research aspects and the numerous references to the international state of the art.  
It is clear that Mr. Degroote masters this subject very well, and is informed very well about the international research activities in this field.

Apart from the scientific quality, it is worth to mention that the quality of the English language is very good, and the layout and style of the manuscript as a whole is impeccable.

***Remarks/comments***

The list below is a selection of some remarks/comments, but does not pretend to be an exhaustive list of the questions that can be posed during the private defence.

- p. 32: the interpolation on the fluid-structure interface is briefly mentioned. Later on in the manuscript, the multi-level algorithms are also discussed. In this context:
  - at the side of the structural solver, it is quite common to use adaptive remeshing during a dynamic simulation. How can the algorithm deal with changing configurations of meshes during one simulation (and not in different simulations such as in the multi-level algorithms),

- now, the finest grid is always considered to be the fluid grid. I can imagine problems in interaction between acoustic waves and solid materials, where you need two to three elements per wavelength in the “fluid” grid, but many more in the solid to detect very little defects in the material. Are there any limitations to the algorithm in that respect ?

- p. 113: for modelling the Mooney-Rivlin material, the used element in ref. [10,218] seems to be a hybrid element, where stresses can be independent degrees of freedom as well.  
Would the algorithm benefit from having hybrid stress elements at the structural solver side, as stress continuity could be imposed more naturally, compared to displacement-based finite elements ?
- p. 121: very little is said about the data transfer between CFD and FEA solvers through the Tango code. Is there a lot of optimization potential in that respect or not ?
- p. 195: the agreement between experiments and simulations for Figure 7.3 is not very convincing. In Figure 7.5c the agreement still seems reasonable, but if one looks at the free water surface in Figure 7.3, the curvature is often opposite to the experimental one. It is difficult to believe that this is only due to the relatively limited knowledge about the rubber properties. Are there other reasons for this disagreement ?
- what happens if during one simulation, the fluid-structure interface breaks up due to failure of the structural component, modelled at the structural solver side. In other words, if fluid breaks through the fluid-structure interface, how does the algorithm deal with that ?
- p. 214: I can of course guess why Fluent was used for this research, but in the conclusions, it is mentioned that one of the drawbacks of Fluent is the first-order accuracy in time. There exist other CFD codes with a second order accuracy in time. It is not justified in the manuscript why Fluent was selected as the best CFD code to do this research.
- although this is not the primary objective of a PhD thesis, it would have been instructive to see a more complex fluid-structure interaction problem on a very large scale. It is likely that the benefits of a partitioned approach would appear much stronger, if a very large and complex problem is dealt with where two dedicated CFD and FEA codes are absolutely needed, compared to the limitations of a monolithic solver. There exist large-scale FSI simulations of bow slamming of large container ships, but of course, the experimental data for validation are not freely accessible due to confidentiality agreements.  
What is the candidate’s opinion in this respect ? Are there any future actions planned in this direction ?
- p. 34: other types of coupled problems are listed here, that have links with research in my group.  
Recently, we had a PhD defence in our research group, where acousto-structural interactions are presented. The “monolithic” simulation in ABAQUS reveals some interesting effects, but real second-order ultrasound-structural interactions are not included. One could imagine to apply the partitioned approach to ultrasound-structural interactions, where the ultrasound wave emits from the fluid (typically water is used as coupling medium) and interacts with the solid. The surface waves that are generated on the surface of the solid, make that the surface is not perfectly flat anymore, but has a sinusoidal profile (although the amplitude is in the order of micrometers or less).

The incident ultrasound beam sees the profile as a corrugation and interference occurs, generating specific diffraction patterns.

Can the algorithm deal with such problems ?

### **Conclusions**

The thesis fulfils the conditions of scientific level and originality. Mr. Degroote can be admitted to the public defence without mandatory changes to the manuscript.

Wim Van Paepegem  
Ghent University  
Department of Materials Science and Engineering
