# Supplementary material for: Faddeev Random Phase Approximation applied to molecules
Source: arXiv:1210.6186 source file (2012-10-23)
Supplement: Supplementary file 6 [file Verstraete.pdf]

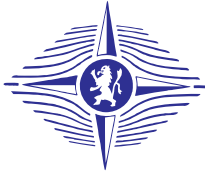

The von Karman Institute for Fluid Dynamics  
Waterloosesteenweg 72  
1640 Sint-Genesius-Rode,  
Belgium

Prof. Luc Taerwe  
c/o Marion Roels  
Faculteit Ingenieurswetenschappen  
Decanaat  
Jozef Plateastraat 22  
BE-9000 Gent

Sint-Genesius-Rode, March 3, 2010

## **Concerns: Evaluation of the PhD thesis of Joris Degroote**

### **“Development of Algorithms for the Partitioned Simulation of Strongly Coupled Fluid-Structure Interaction Problems”**

#### **General description**

This thesis addresses the fluid-structure interaction problem, which allows the simulation of very complicated phenomenon. This technique is gaining interest in recent years, mainly driven by the increased computational available power. However, still a lot of problems need to be addressed. This PhD thesis is situated in the partitioned approach, where two different solvers for the fluid and solid are coupled together to solve the fluid-structure interaction problem.

After a brief introduction, a very dense but yet profound survey of available techniques is provided in a literature review. A third chapter is devoted to the very fundamental stability analysis of the partitioned approach, by looking at a simplified model of the flow in an artery. This stability analysis, excluding in its most simplistic form the inertia in the solid model, allows to understand the instabilities occurring by the coupling. It also concludes that with decreasing time step the instability of the method increases and that by introducing an artificial compressibility term the stability of the method is greatly improved.

The next chapter deals with the coupling of two black-box solvers. A newly developed technique (IQN-ILS) is presented, next to other existing methods. The different

techniques are compared with each other on the test case of a flexible beam and a flexible tube. Then the newly developed technique is compared to a monolithic method for 5 test cases. Only on one case the IQN-ILS performs faster.

A following chapter deals with the coupling of a black-box solver and an accessible solver. A technique is proposed for the partitioned simulation of bubble and droplet dynamics, followed by two examples. The concept of artificial compressibility is introduced by performing 2 fluid computations before the start of the partitioned solution, and is also followed by two examples.

Special techniques to accelerate the partitioned approach were developed and tested for simulations being run on a large parallel scale. The conclusion that the speed-up by using more cores will stall after a certain number of cores has lead to the search for using the parallel capabilities more efficiently. Two techniques have been proposed. The multi-solver technique recalculates the solutions of previous time steps with the current time step situation. However, the efficiency of this technique seems quite poor. The multi-level algorithm computes first the solution on a coarse grid which is used as an initial guess for a finer grid. The later technique seems to have potential to speed up the problem but requires to set-up the problem for different grids, which might increase the set-up effort for the simulation.

The last chapter deals with free surface flows and is illustrated by two examples.

## **General appreciation**

The author has made a profound study of the problem at hand and has made original contributions to several domains. Especially the stability analysis shows that the author surpasses the level of simply trying several methods. Instead, he uses a more profound approach in which he tries to understand why instabilities may occur, why some methods perform better than others and how instabilities can be avoided.

The work presented is complete and very detailed. A very good literature review is given, which is well referenced. The author has made an impressive list of publications.

## **Spelling suggestions:**

The text is very well written and special care was taken by the author to make the text comprehensive. Only very few spelling errors were found and are listed below (but not necessarily limited to those). Some are more suggestions.

- Page 79: “The position of the wall of a tube, which initially has a constant cross-section and contains fluid at rest, ...” Suggestion to add “a” before fluid.
- Page 187: “Multi-phase flow with a free surface can be highly unsteady if waves and droplets are present.” Suggestion to change flow into flows, or “A multi-phase flow”.
- Page 192: “The displacement of the tip of the beam in the rotating reference frame of the tank has been calculated from these images with a computer programme.” Change programme by program.

## Style

It is suggested to make a more clear distinction between text and algorithms in Chapter 2. It would be more practical to refer to those algorithms from the text, also in later parts of the book.

The caption of figures is similar to the body text and leads sometimes to confusing situations. It is suggested to make a more clear distinction by putting for instance the caption in italic, or by intending the text. It is also suggested to reduce the explanations in the captions of the figures to increase the readability of the text.

## Remarks and further questions:

In Chapter 3 a stability analysis for the blood flow in an artery is presented. It is not clear in which way this stability analysis differs from previous work, such as e.g. Causin et al. What are the new contributions of this stability analysis? What is the difference between the model used by the author and other works, and what is the difference in the conclusions drawn?

On Page 42 a pressure stabilization term is introduced. Not being familiar with such a term, what is its influence on the stability analysis? What would happen to the amplification factor if a different value for  $\alpha$  is taken?

On page 44 it is proposed to solve the linearized equation for the solid (Eqn. (3.19)) next to the correct solution of the solid (Eqn. (3.20)). Why would that be done? After convergence of the Gauss-Seidel iterations, the solution will not respect the real solid equations.

On Page 57, Fig. 3.9 the Aitken relaxation method shows an interesting convergence history. Why is it not monotonous, as is the case for the IBQN-LS technique?

On Page 82 it is recommended to exclude the difference between the first vectors in a time step and the last vectors of the previous time step into the matrices V and W. Some reasons for this strategy would be welcome.

On Page 84 the new IQN-ILS method is presented. However, it is not explained why Eqn. (4.21) is an approximation of the Jacobian. Also a proof that it treats low order waves implicitly, as mentioned by the author, is missing. Moreover, to get more insight into the method, it would be interesting to know under which conditions the approximation delivers the correct product with the inverse of the Jacobian in Eqn. (4.21).

The test described in 4.5.2c (the Strong coupling test) is not well explained. It is not clear to unfamiliar people what happens during this test. The fluid-structure interaction tested in this PhD is limited to incompressible flows although here the fluid domain gets compressed almost completely.

Also for the oscillating droplet (section 5.2.4a) the problem is not clearly defined. A sketch of the oscillation of the droplet would help to understand what happens in this test.

On page 141, a pressure adjustment of the outlet is introduced by Eqn. (5.40). It is mentioned in the text that this term is added “to compensate for the change of the bubble volume”. It is not clear why this is necessary, even so how this term is composed.

Although for a partitioned approach the interpolation of data between different grids is very important, this topic is left aside within this work. More details on interpolation and its effect on the results would be welcome.

### **Recommendation**

In conclusion, Mr Degroote has performed an excellent engineering work. It reveals his thorough knowledge of engineering sciences and his ability to perform independent research. This work certainly deserves to be submitted for public defense.

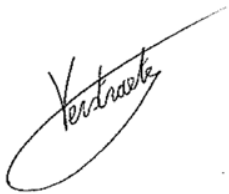A handwritten signature in black ink, reading "Verstraete", enclosed within a large, loopy oval stroke.

Tom Verstraete  
Turbomachinery and Propulsion department.  
von Karman Institute
