# Supplementary material for: Faddeev Random Phase Approximation applied to molecules
Source: arXiv:1210.6186 source file (2012-10-23)
Supplement: Supplementary file 7 [file Wall.pdf]

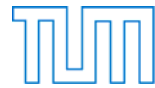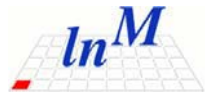

## Evaluation of PhD thesis

### **“Development of Algorithms for the Partitioned Simulation of Strongly Coupled Fluid-Structure Interaction Problems” by Joris Degroote**

#### *Summary*

This thesis is concerned with the development of algorithms for a quite challenging class of problems, namely when flow problems are interacting with structures that exhibit large deformations. This is definitely an up to date topic that has seen a lot of interest in recent years from the international scientific community. The candidate opted for one specific class of algorithms, so called partitioned methods, and develops them further, analyses them and applies them to a variety of problems.

After a short introduction he gives a literature review to set the stage and to present the governing equations and an overview of different methods and approaches.

After that he provides a sort of stability analysis of a Gauss-Seidel type scheme along with a strongly simplified model problem. This gives quite some insight and advice on how to obtain a converging method.

Then he looks into the situation when two black-box solvers have to be coupled. The solution approach adopted here is based on interface quasi-Newton approaches. This approach is discussed in detail and a number of improvements and modifications are suggested. The two main ideas are concentrated on how to get the (approximate) Jacobian (or its' effect) in a cheaper way.

Chpt. 5 considers the situation when only one solver is black-box and the other is accessible. In this setting an approximate model for one solver is introduced into the accessible solver and a faster converging, partially implicit method is used. The classes of problems that are in one case treated with such an idea are bubble and droplet flows. In the other case the previously suggested interface artificial compressibility method is further

analysed and employed. It is also studied how this can be interpreted and formulated as Robin boundary conditions. In chpt. 6 the author looks into multi-solver and multi-level algorithms.

The thesis finishes with an example section where two FSI problems involving free surface flows are calculated.

Finally the work is concluded and some ideas on potential future work are given.

### *Evaluation*

This is definitely a very good thesis. It covers a lot of different aspects on a very challenging subject and it also includes a number of novelties and original ideas. In order to submit such a thesis one needs to have a more than solid background in a number of different fields. The quality of the work is also proven by a number of peer-reviewed journal publications. Honestly, although the thesis covers a number of different aspects and has many interesting parts I however find 11 journal publications inflationary – but this seems to be a common approach nowadays. And this remark also shouldn't damp my overall evaluation of a very good thesis.

In summary, the thesis proves in an impressive way that the candidate is capable of performing independent research on a high international level. I'm therefore very happy to recommend with great emphasis to give Mr. Degroote the permission to the public defence. I have a small number of remarks concerning the work but these are not mandatory and I will use my participation at the public defence to discuss them with the candidate.

Sincerely,

Wolfgang A. Wall
