# Supplementary material for: Faddeev Random Phase Approximation applied to molecules
Source: arXiv:1210.6186 source file (2012-10-23)
Supplement: Supplementary file 8 [file changes.tex]

\chapter{Changes}
\label{app:changes}

\section{Errata}
\label{sec:errata}

\begin{itemize}
	\item \COR{erratumInitialIndex}, below \Equ{structureTimeDiscreteNewmarkPosition}: $i=0,\ldots,N$\\
	$\rightarrow$ $i=1,\ldots,N$.
	\item \COR{erratumMissingDivision}, first paragraph of \Sec{flexibleTube}: Young's modulus 3\EM{5}\,Nm$^2$\\
	$\rightarrow$ Young's modulus 3\EM{5}\,N/m$^2$.
  \item \COR{erratumWrongExponent}, in \Tab{ML-iterations1D-grid}: grid points = $10^3$ on line 1 and 4\\
  $\rightarrow$	grid points = $10^4$ on line 1 and 4.
  \item \COR{errataIsothermalLiterature}, \Cor{errataIsothermalApplications}: unsteady, isothermal flow\\
  $\rightarrow$ unsteady flow.
  \item \COR{errataIsothermalOneBlackBox}: incompressible, isothermal fluid\\
  $\rightarrow$ incompressible fluid.
\end{itemize}

\section{Prof. dr. ir. Hester Bijl}
\label{sec:bijl}

\begin{itemize}
  \item Stability analysis
  	\begin{itemize}
  	  \item Addition of coupling terms\\
  	  	On page 44 of Chapter 3 a stability analysis is performed of Gauss-Seidel partitioning, where information of the elastic wall is added to the flow equations in several places. Would it be possible to do it the other way around, add information on fluid pressures to the structure equation? What would the stability of that type of iteration be compared to the scheme analyzed in the thesis?\\
  	  	$\rightarrow$ The dependence of the radius on the pressure in the structure can be approximated by a local model. However, a local change of the radius will result in a global change of the pressure in the flow solver. Hence, it would require a matrix model (instead of a scalar model) to include the flow into the structure. This can be found in the conclusion of \Cha{oneblackbox}\ on \Cor{bijlFlowInStructure}.
  	  \item Dependence on boundary conditions\\
  	  	How are the boundary conditions taken into account in the stability analysis? Would a change of boundary conditions affect the result?\\
  	  	$\rightarrow$ The boundary conditions are not taken into account. Boundary conditions often prescribe the radius or pressure. As a result, they normally reduce the error amplification, which has also been observed in the numerical experiments. This can be found on \Cor{bijlBoundaryConditions}.
  	  \item Dependence on discretization in space and time\\
  	  	What does the amplification factor for the monolithic system (not the $\mu$ in Eq. (3.27), but the ``standard'' one for the discretization) look like? Is there significant damping for the high frequency modes caused by:
  	  	\begin{itemize}
  	  	  \item the implicit Euler time integration
  	  	  \item the first-order upwind spatial discretization
  	  	  \item the pressure stabilization
  	  	\end{itemize}
  	  	Does the fact that the partitioning is only unstable for low frequency modes depend on this damping of high frequency modes in the discretization? I.e. what would happen when a pure central discretization is used in combination with the trapezoidal rule and no stabilization term? In that case less damping is present for the high frequency modes present, will than also only the low frequency errors be unstable?\\
  	  	$\rightarrow$ In \App{stability}\ on \Cor{bijlInfluenceTimeDiscretization}, the stability analysis is performed with the composite time discretization. The composite scheme divides the time step $\Delta t$ in two sub-steps by means of an intermediate point at $\delta\Delta t$ ($0<\delta<1$) and uses the trapezoidal rule in the first sub-step and the three-point backward Euler scheme in the second sub-step. In the sub-step which uses the trapezoidal rule, the error amplification is almost the same as for the implicit Euler time integration.\\
  	  	In the numerical experiments (e.g. the propagation of a pressure wave in a 3D tube and \Fig{WaveNumber}\ on \Cor{bijlInfluenceSpatialDiscretization}), second-order upwind spatial discretization is used. For that case, it has been observed that the low wave numbers appear first during the coupling iterations so it can be concluded that they are the most unstable modes.\\
  	  	If the pressure stabilization is removed, the high wave numbers become unstable. However, in that case, the flow simulation on its own is also unstable. The pressure wiggles due to the central discretization of the pressure combined with the collocated pressure and velocity grow during a flow simulation in a rigid tube. This has been added on \Cor{bijlInfluencePressureStabilization}.\\
  	\end{itemize}
  \item Multi-solver and multi-level implementation\\
  	Do you have comparisons of MS implementations of IQN-ILS and IBQN-LS with regular implementations? I am interested in more information on the multi-level algorithm. Why did you chose to go from coarse to fine and not use a V-cycle? On page 179 a bias is mentioned in the results when certain terms are added to V and W. Where does this bias come from?\\
  	$\rightarrow$ In a V-cycle, one would first perform iterations on the fine grid. However, during the first coupling iterations, modes with a low wave number will grow because they are the most unstable and no modes are treated implicitly yet. Especially the modes with a low wave number can be captured on a coarse grid at a lower cost than on a fine grid. Therefore, no V-cycle is used but the coupling iterations go from a coarse to a fine grid. This has been added on \Cor{bijlNoVCycle}.\\
  	The bias comes from the change of grid level. On the fine grid level, more details can be resolved than on the coarse grid level. Hence, if the difference between a result on the coarse grid level and a result on the fine grid level is calculated, this contains the actual change but also a change due to the difference in resolution, possibly containing information with a high wave number. This has been added on \Cor{bijlMultiLevelBias}.
\end{itemize}

\section{dr. ir. Philippe Geuzaine}
\label{sec:geuzaine}

\begin{itemize}
  \item p 106: It would be interesting to see the performance of IQN-ILS with no use of previous time-steps.\\
  $\rightarrow$ The simulation of the propagation of a pressure wave has been performed with IQN-ILS and IBQN-LS without reuse and both algorithms require approximately 11 coupling iterations per time step. This has been added in \Tab{resultsTube}\ on \Cor{geuzainePropagationWithoutReuse}.
  \item p 112: How about the memory footprint in Table 4.4?\\
  $\rightarrow$ The IQN-ILS technique requires 20 to 30\,\%\ less memory than the monolithic Newton technique for the propagation of a pressure wave in a flexible tube. This has been added on \Cor{geuzaineMemoryAnalysis}, in \Tab{wavePropagationCost}\ on \Cor{geuzainewavePropagationMemory}\ and in \Tab{wavePropagationLongCost}\ on \Cor{geuzainewavePropagationLongMemory}.
  \item p 112: Could the author elaborate on the use of a limiter?\\
  $\rightarrow$ If the maximal absolute value of the displacement or stress is above a certain threshold, the displacement or stress vector can be rescaled such that its maximal absolute value is equal to that threshold. No limiter has been used for any of the results in this thesis. However, a relaxation factor is used between the first and second coupling iteration if no information from previous time steps is available in the least-squares models. The choice of this relaxation factor is determined by trial and error but usually a value of $\omega=0.01$ works fine. If the coupled problem is very though, it is possible that the flow solver and the structural solver diverge during the second coupling iteration (e.g. because of negative cell volumes in the flow solver) and then $\omega$ has to be reduced manually. This relaxation only takes place between the first and second coupling iteration and hence it is not considered as a limiter which would be active in all coupling iterations. This has been added on \Cor{geuzaineLimiter}
  \item p 115: Could the author add some information for the ``strong coupling'' case?\\
  $\rightarrow$ The strong coupling test consists of an elastic piston in a channel which is filled with an incompressible fluid. The piston is located at the left-hand side of the channel and the velocity on its left-hand side is prescribed as a function of time. At the right-hand side of the channel, an outflow boundary condition with zero normal stress is imposed. This has been added on \Cor{geuzaineStrongCoupling}.
  \item p 145: It would be interesting to compare the results with a VOF approach.\\
  $\rightarrow$ It would indeed be interesting to compare the presented interface-tracking technique with interface-capturing techniques like the volume-of-fluid method. It is expected that the VOF approach will require more grid cells to get a similar resolution of the interface. However, the VOF approach will not require coupling iterations and the pinch-off will be automatic. This has been added as future work on \Cor{geuzaineBubbleVOF}.
  \item p. 166: The licence cost (serial vs. parallel) of commercial solvers could be added to the discussion related to the multisolver version of the algorithms.\\
	$\rightarrow$ Starting a new solver indeed requires a more expensive licence than using an additional core. This has been added on \Cor{geuzaineLicense}.
  \item p. 184: Does the multi-level version of the solvers prove to be more robust?\\
  $\rightarrow$ The aim of the multi-level version is to accelerate and not to make the coupling algorithm more robust. This can be found on \Cor{geuzaineReasonMultiLevel}.
  \item While the list of publications associated with the thesis is impressive, a section in the (introduction or conclusion of the) thesis could gather a summary with the main achievements of them.\\
  $\rightarrow$ The author has chosen to write an outline of the thesis in \Sec{outlineThesis}\ with references to the corresponding papers. Also in the introduction of each chapter, the author refers to the papers on which the chapter is based.
  \item A great emphasis has been put in developing coupling between black-box solvers. This is well motivated from a conceptual point of view. Is it the experience of the author that most solvers do not offer access through user-defined function so that the IAC algorithm (detailed and applied in Chap. 5) cannot be implemented?\\
  $\rightarrow$ To the best of the author's knowledge, most solvers allow for user-defined source terms such that the IAC algorithm can be implemented. This can be found on \Cor{geuzaineUserDefinedSource}.
  \item The thesis focuses mainly on convergence issues. What would be the impact of replacing the first-order time-accurate approach by a second-order one in the flow solver?\\
  $\rightarrow$ \App{stability}\ on \Cor{geuzaineInfluenceTimeDiscretization}\ uses the composite time integration scheme, which is a higher-order scheme. For that scheme, the error amplification is almost the same as for the first-order backward Euler scheme. A higher-order scheme might allow for larger time steps, possibly reducing the number of coupling iterations per time step.
  \item How could the approach be applied to fluid-thermal problems?\\
  $\rightarrow$ Yes, both the fluid and the thermal problem behave in a continuous way, except when phase-changes come into play. Even field-field coupling instead of boundary-boundary coupling is possible. Other coupled problems that might benefit from the algorithms developed in this work can be found in \Sec{otherCoupled}\ on \Cor{geuzaineFluidThermal}.
  \item As the main motivation for partitioned approaches is solver re-usability and the limitation of monolithic solvers to moderate size problems, it would have been nice to demonstrate on a large-scale problem (involving several millions of degrees of freedom) the advantage of partitioned approaches.\\
  $\rightarrow$ The monolithic solver that has been used (ADINA) did at that time not allow to use distributed memory simulations. Hence, it was practically unfeasible. However, this would indeed be very interesting.
\end{itemize}

\section{Prof. dr. ir. Patrick Segers}
\label{sec:segers}

\begin{itemize}
  \item I would suggest to also explain the acronyms in the summary.\\
  $\rightarrow$ The explanation of the acronyms has been added in the summary on \Cor{segersAcronyms}\ and the samenvatting on \Cor{segersAfkortingen}.
  \item Page xiii: ``slagader'' instead of ``ader''.\\
  $\rightarrow$ ``Ader'' has been changed into ``slagader'' on \Cor{segersSlagader}.
  \item Typo p18: $\ldots$ anD that the pressure $\ldots$.\\
  $\rightarrow$ ``An'' has been changed into ``and'' on \Cor{segersAnd}.
  \item Typo p81: start par 2: Newtons.\\
  $\rightarrow$ ``Newtons'' has been changed into ``Newton'' on \Cor{segersNewton}.
  \item Typo p102: $\ldots$ However, its calculation (instead of it's).\\
  $\rightarrow$ ``It's'' has been changed into ``its'' on \Cor{segersIts}.
  \item Section 5.2.1.: add a figure to introduce the coordinate system?\\
  $\rightarrow$ The coordinate system has been added in \Fig{dropletGeometry}\ and \Fig{bubbleGeometry}. Moreover, the inner radius of the needle is indicated as $r_C$ instead of $r$ as this symbol is already used in the coordinate system on \Cor{segersCoordinateSystem}.
  \item Figure 5.6: $P_G$ should be $P_1$?\\
  $\rightarrow$ ``$p_G$'' has been changed into ``$p_1$'' on \Cor{segersPressure}.
  \item P167: for $i=\ldots$ (instead of $0=\ldots$).\\
  $\rightarrow$ ``$0$'' has been changed into ``$i$'' on \Cor{segersIndex}.
\end{itemize}

\section{Prof. dr. ir. Wim Van Paepegem}
\label{sec:vanpaepegem}

\begin{itemize}
  \item p. 32: the interpolation on the fluid-structure interface is briefly mentioned. Later on in the manuscript, the multi-level algorithms are also discussed. In this context:
  \begin{itemize}
    \item at the side of the structural solver, it is quite common to use adaptive remeshing during a dynamic simulation. How can the algorithm deal with changing configurations of meshes during one simulation (and not in different simulations such as in the multi-level algorithms),\\
    $\rightarrow$ It is also common to use adaptive remeshing of the fluid grid during a dynamic simulation. Although in this work no adaptive remeshing was used in the structural grid, it has extensively been used in the fluid grid. Therefore, no fundamental difficulties are expected due to dynamic adaptive remeshing in the structural grid. This has been added on \Cor{vanPaepegemAdaptiveRemeshing}.
    \item now, the finest grid is always considered to be the fluid grid. I can imagine problems in interaction between acoustic waves and solid materials, where you need two to three elements per wavelength in the ``fluid'' grid, but many more in the solid to detect very little defects in the material. Are there any limitations to the algorithm in that respect?\\
    $\rightarrow$ No difficulties are expected for the coupling algorithms if the solid grid were the finest grid. However, the current interpolation techniques have not been tested for very large differences between the number of points on both sides of the fluid-structure interface but other interpolation techniques can be implemented without influencing the coupling algorithms. This has been added on \Cor{vanPaepegemDifferenceMeshes}.
  \end{itemize}
  \item p. 113: for modelling the Mooney-Rivlin material, the used element in ref. [10,218] seems to be a hybrid element, where stresses can be independent degrees of freedom as well. Would the algorithm benefit from having hybrid stress elements at the structural solver side, as stress continuity could be imposed more naturally, compared to displacement-based finite elements?\\
  $\rightarrow$ The stress on the solid side of the fluid-structure interface is an input and not an output of the structural solver. So, it is not expected that the coupling iterations would converge faster due to the continuity of the stress inside the structural solver.
  \item p. 121: very little is said about the data transfer between CFD and FEA solvers through the Tango code. Is there a lot of optimization potential in that respect or not?\\
  $\rightarrow$ Tango did not have to perform any interpolation for the tests with ADINA in \Sec{numericalStudies}. All interpolation was performed by ADINA so that Tango worked between conformal grids. This can be found on \Cor{vanPaepegemInterpolationADINA}. Nevertheless, the interpolation techniques in Tango as described in \App{tango}\ are simple and there is indeed potential for improvement in that domain.
  \item p. 195: the agreement between experiments and simulations for Figure 7.3 is not very convincing. In Figure 7.5c the agreement still seems reasonable, but if one looks at the free water surface in Figure 7.3, the curvature is often opposite to the experimental one. It is difficult to believe that this is only due to the relatively limited knowledge about the rubber properties. Are there other reasons for this disagreement?\\
  $\rightarrow$ A similar difference between the experiment and monolithic PFEM simulations is observed in \cite{Idelsohn2008b}. A small difference in the deflection of the beam means that the fluid will either touch beam or flow underneath it. This difference will subsequently influence the structural deflection, etc. Consequently, a small difference in the material properties can have a large effect at the end of the simulation.
  \item What happens if during one simulation, the fluid-structure interface breaks up due to failure of the structural component, modelled at the structural solver side. In other words, if fluid breaks through the fluid-structure interface, how does the algorithm deal with that?\\
  $\rightarrow$ This would be very difficult to solve. Depending on the stress on the structure, the structure will either fail or not in a given time step. Hence, the relation between the structural displacement and the stress on the structure will be nonlinear and discontinuous within a time step. This cannot be represented accurately by a linear least-squares model. Another approximation for the product of the Jacobian with a vector would have to be constructed or the data in the least-squares model should be discarded when the behaviour of the structure changes. Apart from that, it would be very difficult to perform such a simulation with a moving grid flow solver. The fluid grid would have to get into the crack in some way. Nevertheless, the geometry changes in \Sec{BubbleGrowthAndDetachment}\ where the bubble detaches from the needle. In that simulation, the break-up was not really simulated. The simulation was stopped when the bubble had almost detached from the needle, but it was still connected to the needle in each coupling iteration of the last time step. The separation was performed manually and then the simulation was resumed.
  \item p. 214: I can of course guess why Fluent was used for this research, but in the conclusions, it is mentioned that one of the drawbacks of Fluent is the first-order accuracy in time. There exist other CFD codes with a second order accuracy in time. It is not justified in the manuscript why Fluent was selected as the best CFD code to do this research.\\
  $\rightarrow$ No quantitative or qualitative comparison between Fluent and other CFD codes was performed at the beginning of this research. The most important aspects for this choice were that a lot of experience with Fluent (User Defined Functions, Scheme, getting/setting values, $\ldots$) was available in the research group, that Fluent is user-friendly and that licences were available at the start of the research.
  \item although this is not the primary objective of a PhD thesis, it would have been instructive to see a more complex fluid-structure interaction problem on a very large scale. It is likely that the benefits of a partitioned approach would appear much stronger, if a very large and complex problem is dealt with where two dedicated CFD and FEA codes are absolutely needed, compared to the limitations of a monolithic solver. There exist large-scale FSI simulations of bow slamming of large container ships, but of course, the experimental data for validation are not freely accessible due to confidentiality agreements. What is the candidate’s opinion in this respect? Are there any future actions planned in this direction?\\
  $\rightarrow$ This would indeed be a nice application. No problems are expected for the coupling algorithms but probably the result will strongly depend on the quality of the flow solver. Therefore, it would be necessary to analyze a number of flow solvers and compare their performance and accuracy for free surface flow.
  \item p. 34: other types of coupled problems are listed here, that have links with research in my group. Recently, we had a PhD defence in our research group, where acousto-structural interactions are presented. The ``monolithic'' simulation in ABAQUS reveals some interesting effects, but real second-order ultrasound-structural interactions are not included. One could imagine to apply the partitioned approach to ultrasound-structural interactions, where the ultrasound wave emits from the fluid (typically water is used as coupling medium) and interacts with the solid. The surface waves that are generated on the surface of the solid, make that the surface is not perfectly flat anymore, but has a sinusoidal profile (although the amplitude is in the order of micrometers or less). The incident ultraound beam sees the profile as a corrugation and interference occurs, generating specific diffraction patterns. Can the algorithm deal with such problems?\\
  $\rightarrow$ If acoustics are involved, the water has to be modelled as compressible. For compressible fluids, a local displacement of the interface leads to a local compression/expansion of the fluid instead of a global acceleration/deceleration for an incompressible fluid. Therefore, cases with compressible fluids are relatively easy for the coupling algorithms. This has been added on \Cor{vanPaepegemAcousticsStructure}.
\end{itemize}

\section{Prof. dr. ir. Tom Verstraete}
\label{sec:verstraete}

\subsection{Spelling suggestions}

\begin{itemize}
  \item Page 79: ``The position of the wall of a tube, which initially has a constant cross-section and contains fluid at rest, $\ldots$'' Suggestion to add ``a'' before fluid.\\
  $\rightarrow$ ``Fluid'' has been changed into ``a fluid'' on \Cor{verstraeteAddA}.
  \item Page 187: ``Multi-phase flow with a free surface can be highly unsteady if waves and droplets are present.'' Suggestion to change flow into flows, or ``A multi-phase flow''.\\
  $\rightarrow$ ``Multi-phase flow'' has been changed into ``a multi-phase flow'' on \Cor{verstraeteAddAAgain}.
  \item Page 192: ``The displacement of the tip of the beam in the rotating reference frame of the tank has been calculated from these images with a computer programme.'' Change programme by program.\\
  $\rightarrow$ British-English spelling has been used throughout this thesis, so this has not been changed.
\end{itemize}

\subsection{Style suggestions}

\begin{itemize}
  \item It is suggested to make a more clear distinction between text and algorithms in Chapter 2. It would be more practical to refer to those algorithms from the text, also in later parts of the book.\\
  $\rightarrow$ The algorithms in \Cha{literature}\ and \Cha{stability}\ have been changed. Their style is identical to the algorithms in the other chapters (e.g. \Cha{twoblackbox}) and they appear in the \listalgorithmname.
  \item The caption of figures is similar to the body text and leads sometimes to confusing situations. It is suggested to make a more clear distinction by putting for instance the caption in italic, or by intending the text. It is also suggested to reduce the explanations in the captions of the figures to increase the readability of the text.\\
  $\rightarrow$ The captions have been changed. The label is bold and the text is indented. The length of the text has not been reduced but the font size is smaller.
\end{itemize}

\subsection{Remarks and further questions}

\begin{itemize}
  \item In Chapter 3 a stability analysis for the blood flow in an artery is presented. It is not clear in which way this stability analysis differs from previous work, such as e.g. Causin et al. What are the new contributions of this stability analysis? What is the difference between the model used by the author and other works, and what is the difference in the conclusions drawn?\\
  $\rightarrow$ The first two paragraphs on \Cor{verstraeteDifferenceStability}\ describe the difference between the analysis in \Cha{stability}\ and the literature. The contribution of \Cha{stability}\ compared to the literature is the Fourier decomposition of the error, which leads to the conclusion that only a fraction of the modes is unstable.\\
  \citet{Forster2007}\ use a variant of the lid-driven cavity problem with a flexible bottom and they include the fluid viscosity in their analysis. \citet{Causin2005}\ analyze the flow in a straight tube comparable to the model in \Cha{stability}\ but two-dimensional and two-dimensional axisymmetric instead of one-dimensional. \citet{Badia2008}\ refer to \citet{Causin2005}\ for the description of the model.\\
  It is not possible to compare with the conclusions of \citet{Forster2007}\ as they do not analyze coupling iterations. The comparison with the conclusions of \citet{Causin2005}\ can be found on \Cor{verstraeteDifferenceConclusion}\ for independent tube segments without structural inertia and has been added on \Cor{verstraeteAddedComparison}\ for the interacting tube segments with structural inertia. In \Sec{robin}, the Interface Artificial Compressibility technique is compared with Robin boundary conditions as used by \citet{Badia2008}.
  \item On Page 42 a pressure stabilization term is introduced. Not being familiar with such a term, what is its influence on the stability analysis? What would happen to the amplification factor if a different value for $\alpha$ is taken?\\
  $\rightarrow$ If the pressure stabilization is removed, the high wave numbers become unstable. However, in that case, the flow simulation on its own is also unstable. The pressure wiggles due to the central discretization of the pressure combined with the collocated pressure and velocity grow during a flow simulation in a rigid tube. This has been added on \Cor{verstraeteInfluencePressureStabilization}.
	\item On page 44 it is proposed to solve the linearized equation for the solid (Eqn. (3.19)) next to the correct solution of the solid (Eqn. (3.20)). Why would that be done? After convergence of the Gauss-Seidel iterations, the solution will not respect the real solid equations.\\
  $\rightarrow$ It is not proposed to solve \Equ{constitutiveStabilized}\ next to \Equ{constitutiveNonLinearStabilized}, but only one of them, \Equ{constitutiveStabilized}\ or \Equ{constitutiveNonLinearStabilized}. This has been emphasized by adding ``either'' on \Cor{verstraeteOnlyOneStructure}.\\
  If the linearized equation for the solid is used in the Gauss-Seidel iterations and the same linearized equation is substituted into the flow equations, then the problem is in fact solved in a monolithic way. Hence, the coupling iterations have to converge in one iteration if all substitution terms are enabled ($\gamma_1=\gamma_2=\gamma_3=\gamma_4=1$). This is explained on \Cor{verstraeteReasonLinearizedStructure}.
  \item On Page 57, Fig. 3.9 the Aitken relaxation method shows an interesting convergence history. Why is it not monotonous, as is the case for the IBQN-LS technique?\\
  $\rightarrow$ In the literature, the convergence of the coupling iterations with Aitken relaxation is given for a lid-driven cavity with a flexible bottom \cite{Kuttler2008}. This problem is shown in \Fig{aitkenCavityDescription}. The convergence behaviour of Aitken relaxation for this case is also not monotone, as can be seen in \Fig{aitkenCavityConvergence}. However, no explanation is known for this behaviour.

  \begin{figure}
		\begin{center}
	  	\includegraphics[width=0.5\textwidth, trim=0cm 7.5cm 0cm 7.0cm, clip=true]{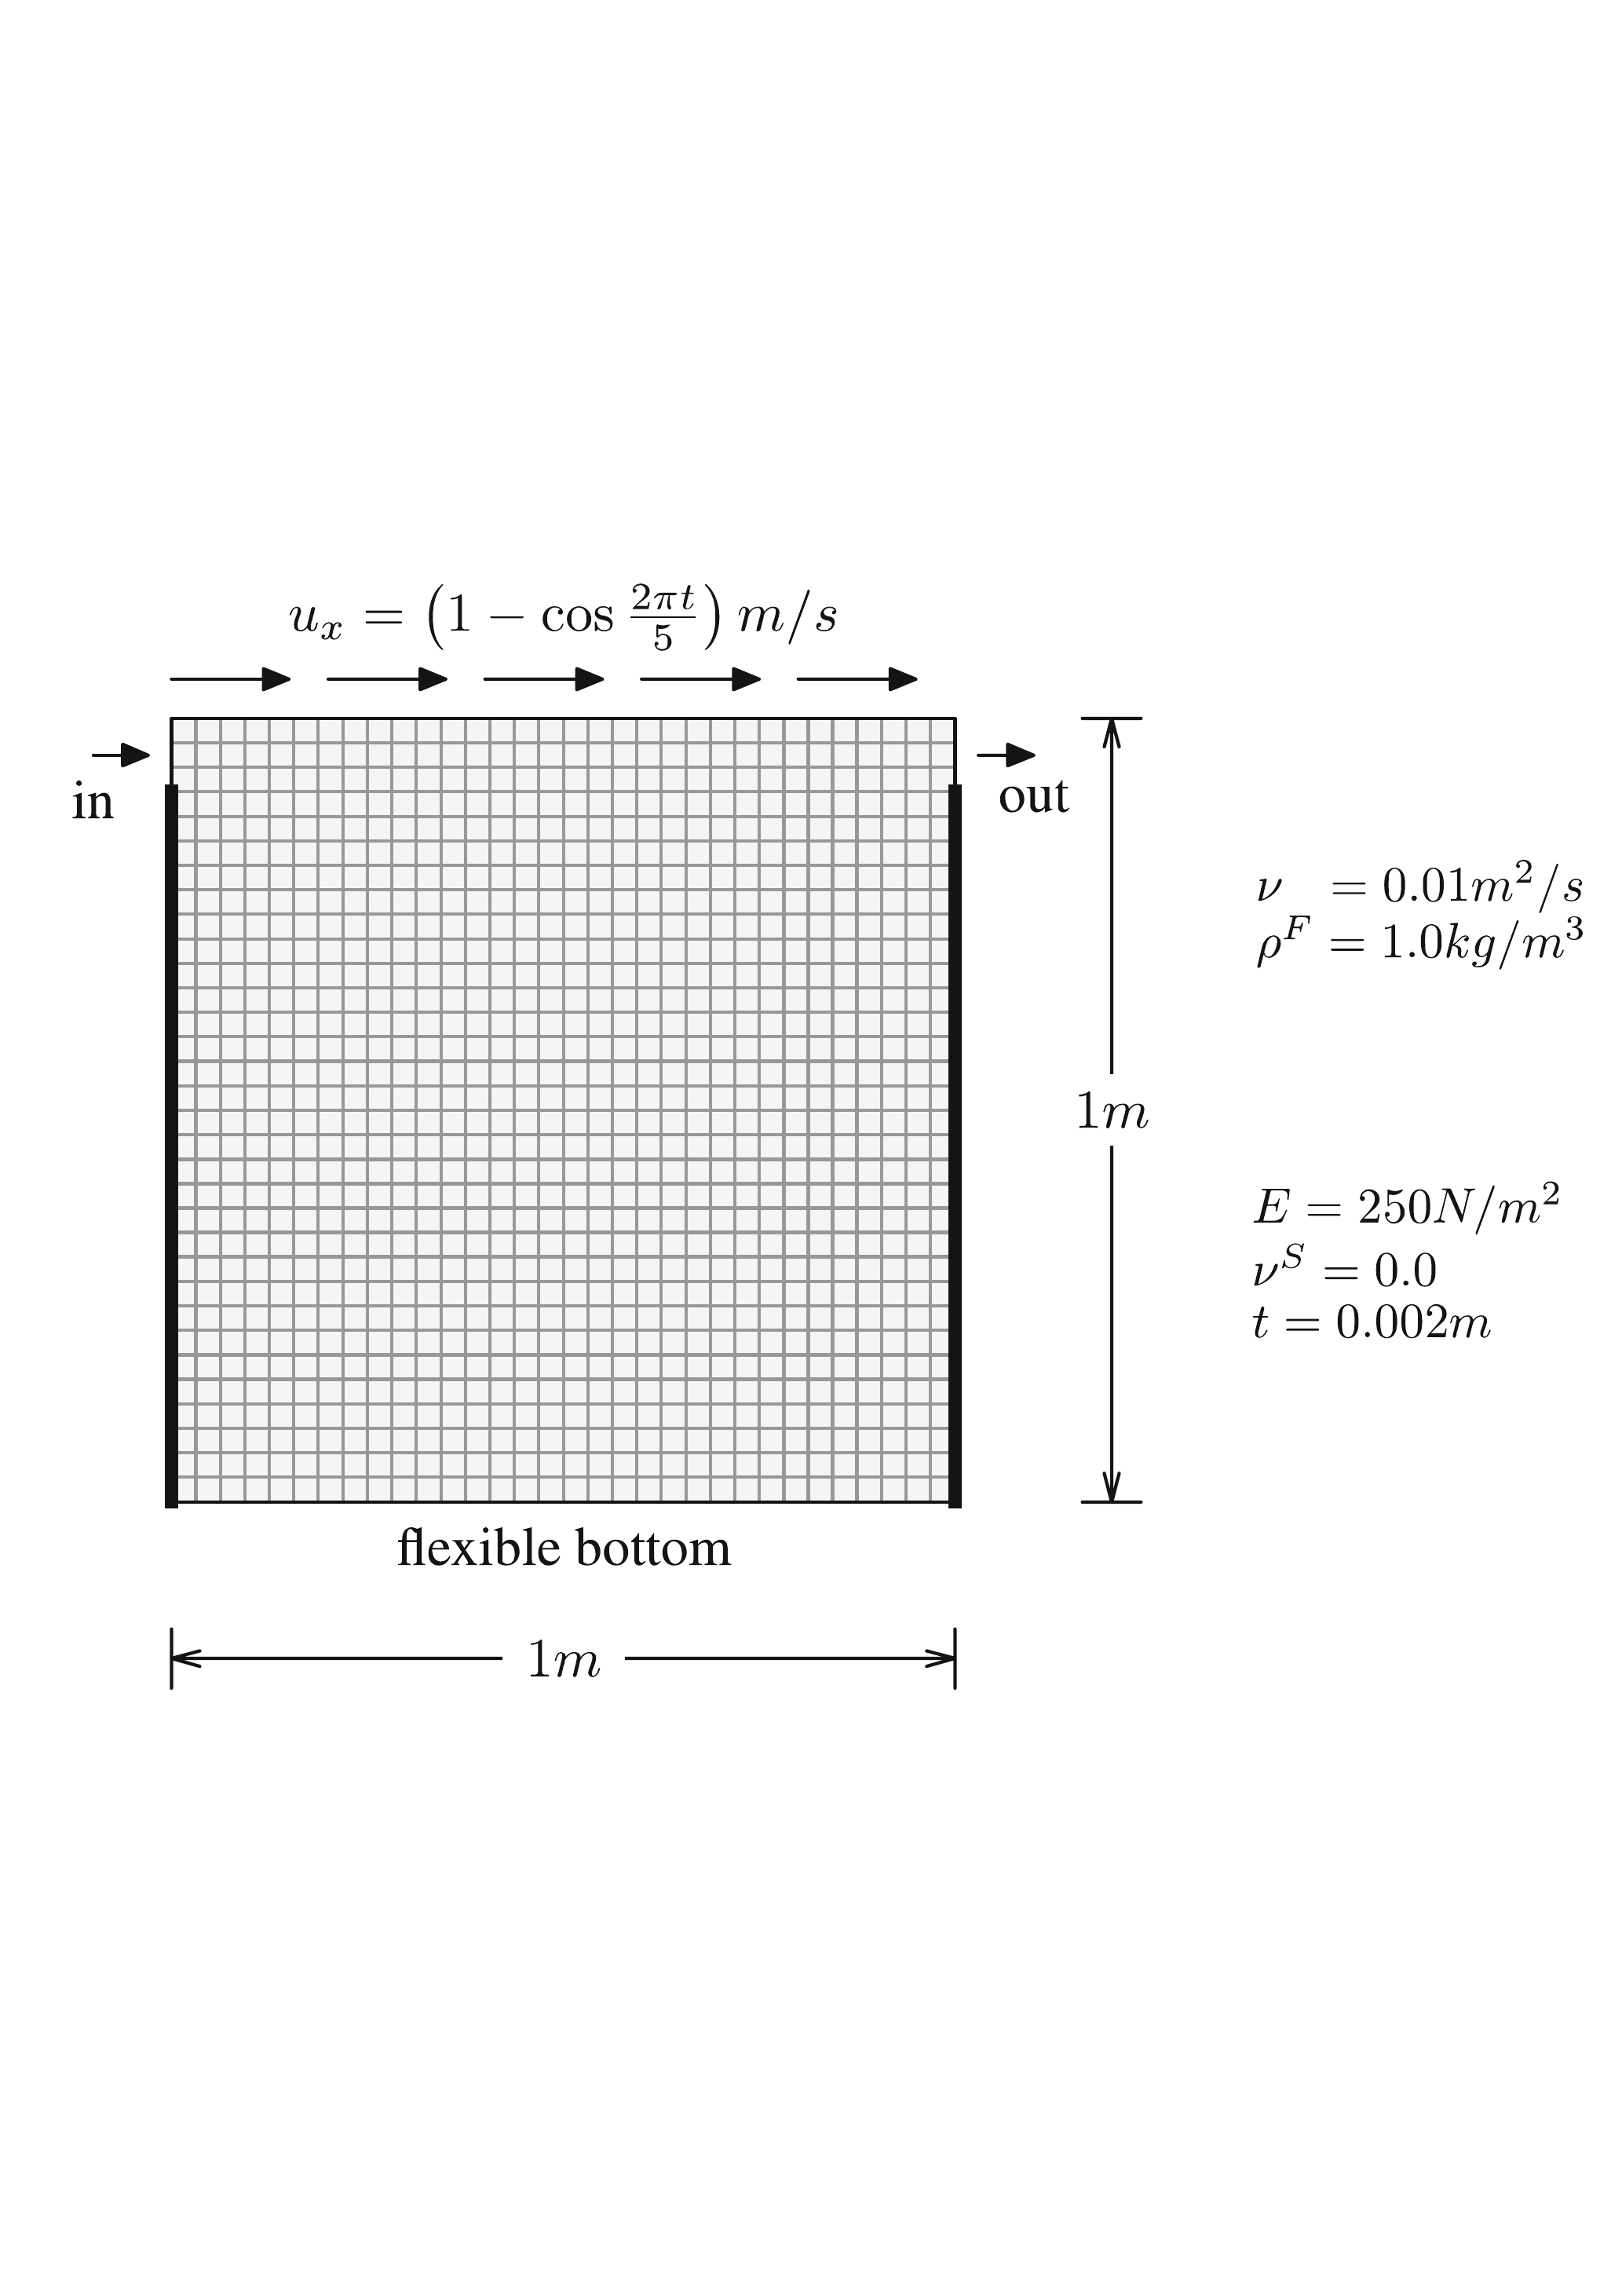}
		\end{center}
		\caption[The model for the lid-driven cavity with a flexible bottom.]{
			\label{fig:aitkenCavityDescription}
			The model for a lid-driven cavity with a flexible bottom \cite{Kuttler2008}.
		}
	\end{figure}

	\begin{figure}
		\begin{center}
	  	\includegraphics[width=0.5\textwidth, trim=0cm 8.4cm 0cm 8.4cm, clip=true]{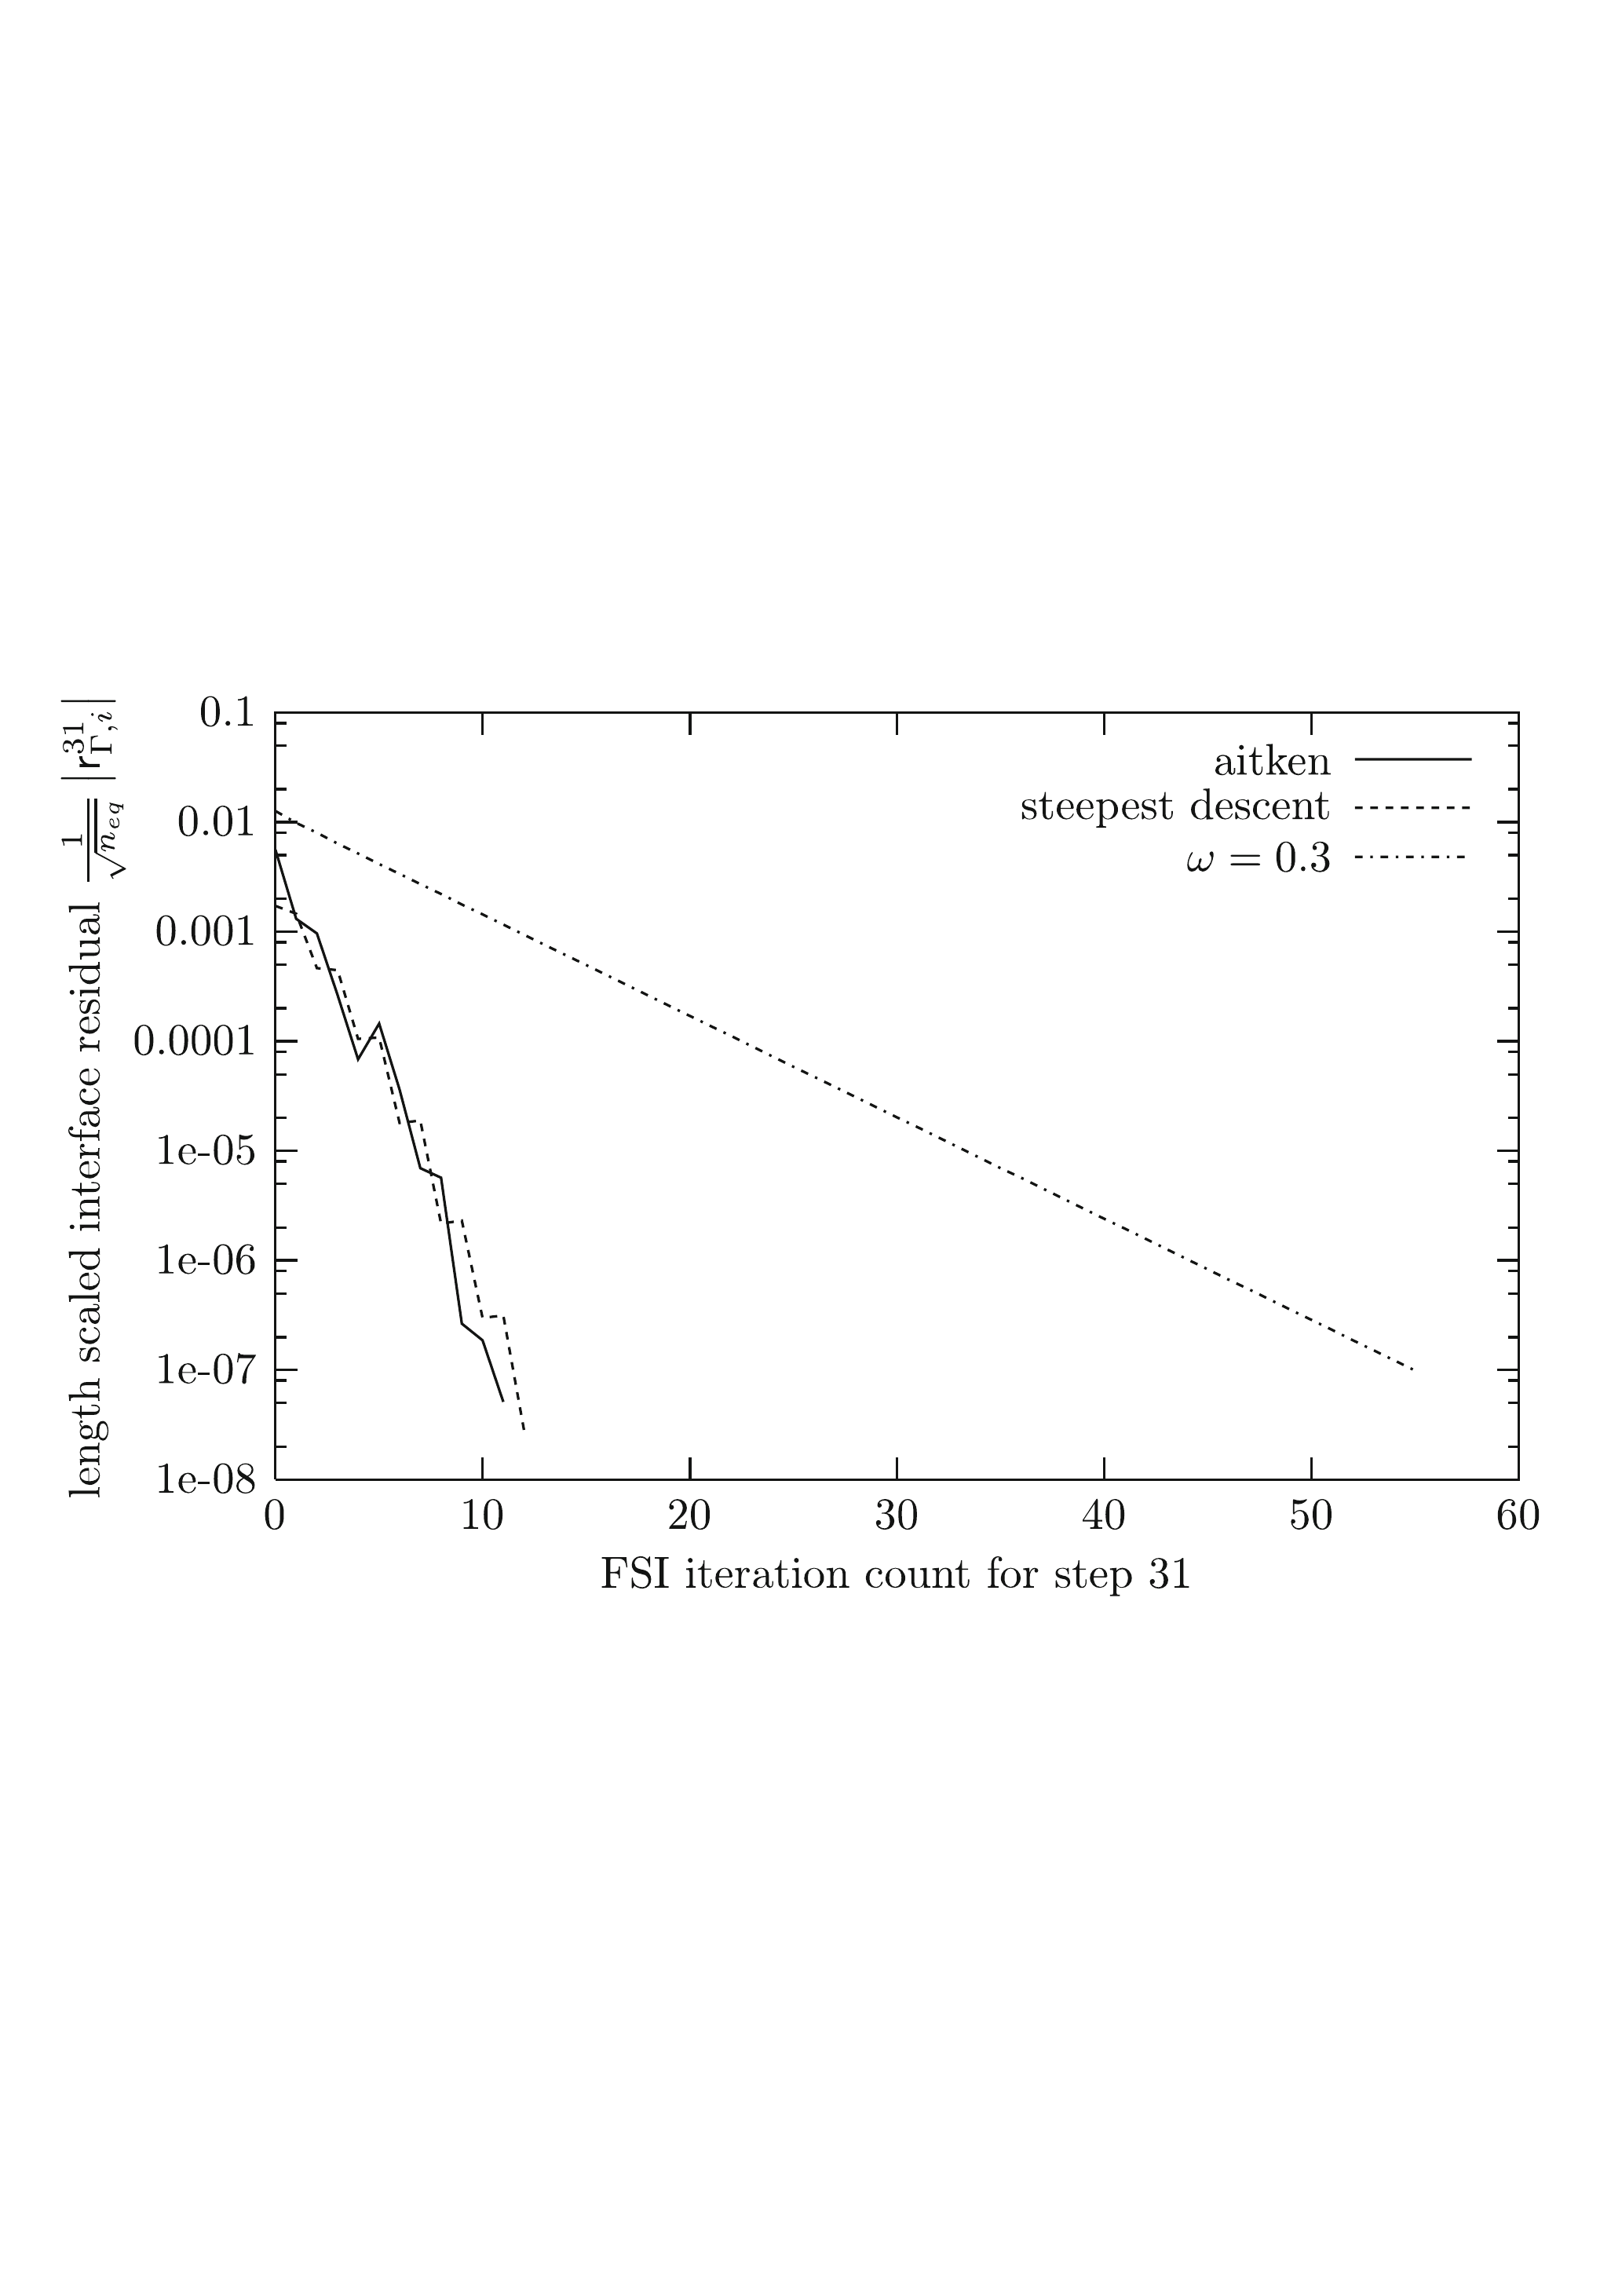}
		\end{center}
		\caption[The convergence of the coupling iterations for the lid-driven cavity with a flexible bottom.]{
			\label{fig:aitkenCavityConvergence}
			The convergence of the coupling iterations for the lid-driven cavity with a flexible bottom and $\rho_s=50$\,kg/m$^3$ \cite{Kuttler2008}.
		}
	\end{figure}

  \item On Page 82 it is recommended to exclude the difference between the first vectors in a time step and the last vectors of the previous time step into the matrices V and W\@. Some reasons for this strategy would be welcome.\\
  $\rightarrow$ It should be noted that ${\res'}^k$ is the Jacobian of $\vt{r}^k$ with respect to $\vt{x}^k$, all at time level $n+1$. If differences between vectors from different time levels are used, then a time derivative is included while ${\res'}^k$ relates differences \emph{within}\ a time step. This has been added on \Cor{verstreateDifferenceOverTimeStep}.
  \item On Page 84 the new IQN-ILS method is presented. However, it is not explained why Eqn. (4.21) is an approximation of the Jacobian. Also a proof that it treats low order waves implicitly, as mentioned by the author, is missing. Moreover, to get more insight into the method, it would be interesting to know under which conditions the approximation delivers the correct product with the inverse of the Jacobian in Eqn. (4.21).\\
  $\rightarrow$ For a vector $\Delta\vt{r}$ in the subspace spanned by the columns of $\mt{V}^k$, the IQN-ILS algorithm is a finite difference approximation for Newton iterations. For a vector $\Delta\vt{r}$ orthogonal to that subspace, Gauss-Seidel iterations are performed. This has been explained in more detail on \Cor{verstraeteProveImplicit}.\\
  As the error modes with a low wave number have an error amplification larger than one (see \Cha{stability}), they appear in the residual during the first coupling iterations. Once a mode has appeared, it is in the subspace spanned by the columns of $\mt{V}^k$. Hence, IQN-ILS switches from Gauss-Seidel iterations (which are not working as the mode appeared in the residual) to quasi-Newton iterations for this mode.
  \item The test described in 4.5.2c (the Strong coupling test) is not well explained. It is not clear to unfamiliar people what happens during this test. The fluid-structure interaction tested in this PhD is limited to incompressible flows although here the fluid domain gets compressed almost completely.\\
  $\rightarrow$ The strong coupling test consists of an elastic piston in a channel which is filled with an incompressible fluid. The piston is located at the left-hand side of the channel and the velocity on its left-hand side is prescribed as a function of time. At the right-hand side of the channel, an outflow boundary condition with zero normal stress is imposed. This has been added on \Cor{verstraeteStrongCoupling}.
  \item Also for the oscillating droplet (section 5.2.4a) the problem is not clearly defined. A sketch of the oscillation of the droplet would help to understand what happens in this test.\\
  $\rightarrow$ The droplet is initially non-spherical (see \Fig{dropletDescription}) so it will start to oscillate. The oscillation amplitude will reduce due to the fluid viscosity. Finally, the droplet will become a sphere. This explanation and \Fig{dropletDescription}\ which shows the vertical position of the top of the droplet as a function of time have been added on \Cor{verstraeteDroplet}.
  \item On page 141, a pressure adjustment of the outlet is introduced by Eqn. (5.40). It is mentioned in the text that this term is added ``to compensate for the change of the bubble volume''. It is not clear why this is necessary, even so how this term is composed.\\
  $\rightarrow$ Initially, the water level is flush with the top of the computational domain. However, as the bubble grows, water is pushed out at the top of the computational domain. Hence, the pressure at the top of the computational domain has to be increased by the height of the water above the top of the domain multiplied by $\rho_2 \cdot g$. This explanation and \Fig{bubbleOutlet}\ have been added on \Cor{verstreateOutlet}.
  \item Although for a partitioned approach the interpolation of data between different grids is very important, this topic is left aside within this work. More details on interpolation and its effect on the results would be welcome.\\
  $\rightarrow$ The interpolation of data between different grids is equally important in the partitioned and the monolithic approach. If non-matching grids are used in a monolithic simulation, appropriate interpolation is also required. Interpolation is however a completely different topic (e.g. A.~de Boer, Computational fluid-structure interaction. Spatial coupling, shell and mesh deformation. Technische Universiteit Delft, 2008.) that can be studied separately from the coupling algorithms which are the focus of this thesis. Initially, conformal meshes were used so there was no interpolation at all. Later, simple interpolation techniques as described in \Sec{interpolation}\ have been implemented to allow for non-matching grids. These simple interpolation techniques do not require access to the discretization in the solvers, which is in lign with the fact that also the coupling algorithms treat the solvers as black boxes. Several simulations (e.g. the propagation of a pressure wave in a straight 3D tube in \Sec{flexibleTube}) have been performed with matching and non-matching grids and no significant differences have been found.
\end{itemize}
